# Supplementary material for: Vector-Valued Gaussian Processes and their Kernels on a Class of Metric Graphs
Source: arXiv:2501.10208 source file (2025-01-17)
Supplement: Supplementary file 1 [file Supplement.tex]

% \begin{supplement}
%     \stitle{Technical Results and Proofs}
%     \sdescription{This supplementary material contains proofs and technical results. To help the reader, Figure \ref{fig:resultsRoadMap} provides the road-map of the main results of this manuscript.}

% \end{supplement}
% \begin{supplement}
%     \stitle{A Worked Example}
%     \sdescription{
% \end{supplement}
